# Supplementary material for: TACO: Tackling Over-correction in Federated Learning with Tailored Adaptive Correction
Source: arXiv:2504.17528 source file (2025-04-24)
Supplement: Supplementary file 1 [file full_appendix.tex]

\begin{appendices}
\allowdisplaybreaks[3]
